# Supplementary material for: Physiome-ODE: A Benchmark for Irregularly Sampled Multivariate Time Series Forecasting Based on Biological ODEs
Source: arXiv:2502.07489 source file (2026-05-22)
Supplement: Supplementary file 1 [file ethics_license.tex]

\section{Societal Impact}\label{sec:ethics}
In this paper we present \Bench, a benchmark designed for IMTS forecasting.
We hope, that our work can contribute to future research in that field.
We do not see any possible negative impact on society.

\section{Licenses}\label{sec:licenses}
The Physiome Repository~\citep{Yu2011.Physiome} is licensed under three
licenses: GPL, LGPL and MPL\@.
For further information see \url{https://models.physiomeproject.org/about/pmr2}.
Our data does not contain any personally identifiable information or offensive
content.
