# Supplementary material for: Physiome-ODE: A Benchmark for Irregularly Sampled Multivariate Time Series Forecasting Based on Biological ODEs
Source: arXiv:2502.07489 source file (2026-05-22)
Supplement: Supplementary file 2 [file regular_MTS.tex]

\begin{table}
\begin{tabular}{lll}
	\toprule
	Name & actually multivariate & remark
\\	\midrule
	FRED-MD & No & Only one time series
\\	NN5  & NO & Forecast Cash withdrawal of different ATMs
\\	Solar & No & Forecast Power in different solar plants every 10 mins over a year
\\	COVID Deaths & Yes
\\	Electricity & No
\\	San Francisco Traffic & NO & just the occupation (can be spatial temporal)
\\	Rideshare & Yes
\\	Web Traffic	& No & Clicks on some Wikipedia article
\\	Car Parts & NO & sales 2674 different over 51 months
\\	Temperature Rain & Yes & 2 channels
\\	\bottomrule
\end{tabular}
\end{table}
